# Supplementary material for: Representation Projection Invariance Mitigates Representation Collapse
Source: arXiv:2205.11603 source file (2023-11-21)
Supplement: Supplementary file 2 [file cka.tex]

\section{Centered Kernel Alignment}\label{sec:cka}
