# Supplementary material for: Representation Projection Invariance Mitigates Representation Collapse
Source: arXiv:2205.11603 source file (2023-11-21)
Supplement: Supplementary file 3 [file concort_capcort_comparison.tex]

\section{\concort vs \capcort}\label{sec:concort_vs_capcort}
