# Supplementary material for: Representation Projection Invariance Mitigates Representation Collapse
Source: arXiv:2205.11603 source file (2023-11-21)
Supplement: Supplementary file 4 [file dataset_description.tex]

\section{Dataset description}\label{sec:dataset_description}

GLUE benchmark contains seven tasks, which cover paraphrase detection (MRPC, QQP), natural language inference (MNLI, RTE, QNLI), linguistic acceptability (CoLA) and sentiment classification (SST-2). We also assembled non-GLUE benchmark from six distinct tasks which include biomedical relation extraction on  CHEMPROT~\citep{KringelumKBLOT16}, sentiment classification on  YELP~\citep{ZhangZL15} and IMDB~\citep{MaasDPHNP11}, citation intent classification on SCICITE~\citep{CohanWMF19}, language inference on SCITAIL~\citep{TusharAP18} and article topic classification on AGNEWS~\citep{XiangJY15}.
