# Supplementary material for: Representation Projection Invariance Mitigates Representation Collapse
Source: arXiv:2205.11603 source file (2023-11-21)
Supplement: Supplementary file 5 [file hpo.tex]

\section{Learning rate and Epochs as hyper-parameters}\label{sec:hpo_lr_epochs}
Table~\ref{tab:hpo_lr_epochs} discusses the results when we search over optimal learning rate and number of epochs for each task and method. For learning rate, we perform the search over [5e-6,1e-5,2e-5,4e-5] and for epochs, we search over [5,10].
\begin{table*}[ht]
\begin{tabular}{lccccccc}
\toprule
       Tasks & STD++ &                  DA &                  WC & ReInit &   R3F &             \concort &             \capcort \\
\midrule
     qqp-10k &  78.58 &  78.79 &  78.20 &  78.74 &  78.67 &  {\bf 79.71} &  79.23 \\
rte &  72.92 &  74.45 &  74.30 &  74.11 &  74.20 &  {\bf 75.09} &  74.95 \\
        cola &  56.67 &  62.36 &  61.79 & 61.50 &  61.74 &  {\bf 62.45} &  61.82 \\
        mrpc &  90.30 &  90.50 &  90.44 &  90.79 &   90.41 &  90.79 &  {\bf 90.83} \\
\bottomrule
\end{tabular}
\caption{Results with HPO over epochs and learning rate}
\label{tab:hpo_lr_epochs}
\end{table*}
