# Supplementary material for: Representation Projection Invariance Mitigates Representation Collapse
Source: arXiv:2205.11603 source file (2023-11-21)
Supplement: Supplementary file 6 [file longer_training.tex]

\section{Longer training with \stdpp}\label{sec:longer_training}
