# Supplementary material for: Representation Projection Invariance Mitigates Representation Collapse
Source: arXiv:2205.11603 source file (2023-11-21)
Supplement: Supplementary file 7 [file stdpp.tex]

\section{STANDARD++}\label{sec:stdpp}
