# Supplementary material for: Representation Projection Invariance Mitigates Representation Collapse
Source: arXiv:2205.11603 source file (2023-11-21)
Supplement: Supplementary file 8 [file top_intermediate_smooth_concort.tex]

\section{\concort - Top Layer vs Intermediate Layer vs All Layers}\label{sec:smooth_intermediate_emb}
