# Supplementary material for: Representation Projection Invariance Mitigates Representation Collapse
Source: arXiv:2205.11603 source file (2023-11-21)
Supplement: Supplementary file 9 [file weight_consolidation_relation.tex]

\section{Relation to Weight Consolidation}
\label{sec:weight_consolidation_comparison}
Apart from working with representations instead of model weights, key difference between our method and weight consolidation is the following: {\em our method tries to control the structural change in representations and does not always keep fine-tuned representations close to the pre-trained representations}. Regularizing fine-tuned representations to be close to pre-trained representations is just a special case and the most strict form of our method (\concort).  The knob ($\Phi$) in our method can be selected to chose a regularizer ranging from this extreme case to the other extreme case with no regularization. Note that this knob is not same as the regularization constant which is used to weigh regularization loss compared to cross-entropy loss.
\danielk{I suggest we bring the above paragraph to the main text.}
